# Supplementary material for: Exact Recovery of Tensor Robust Principal Component Analysis under Linear Transforms
Source: arXiv:1907.08288 source file (2019-07-16)
Supplement: Supplementary file 1 [file MACPdef-ams_supp.tex]

% Definitions that require the amsmath.sty and amsthm.sty files
% Time-stamp: <07/01/15 18:05:06 miguel>

% -------------- Operators --------------

% Probability

% Functions

% Information theory

%\newcommand{\KLop}{\operatorname{KL}}
 % Kullback-Leibler divergence
   % Symmetrised KL divergence
%\newcommand{\inproduct}[2]{\left\langle#1,#2\right\rangle}  % inner product

% Set theory
% Are "card" and "im" the correct names in English?

% Matrices

           % Cofactor of a matrix element
           % Adjunt matrix

% -------------- Theorem environments --------------
%\theoremstyle{plain}% default
%[section]

%\newtheorem*{lemma*}{Lemma}

%\newtheorem*{prop*}{Proposition}

%
%\theoremstyle{definition}
%[section]
%\newtheorem*{defn*}{Definition}
%\newtheorem{exmp}{Example}[section]
%\newtheorem*{exmp*}{Example}
%\newtheorem{conj}{Conjecture}[section]
%\newtheorem*{conj*}{Conjecture}
%
%\theoremstyle{remark}
%\newtheorem{rmk}[thm]{Remark}
%\newtheorem*{rmk*}{Remark}

%%% Local Variables: 
%%% mode: plain-tex
%%% TeX-master: t
%%% End: 
